# Supplementary material for: Diagnostics of cognitive failures in multi-agent expert systems using dynamic evaluation protocols and subsequent mutation of the processing context
Source: arXiv:2509.15366 source file (2025-09-18)
Supplement: Supplementary file 1 [file appendix_table.tex]

\begin{table}[!h]
    \centering
    \begin{tabular}{c|c}
        5 & 6 \\
        7 & 8
    \end{tabular}
    \caption{Caption}
    \label{table:appendix_introduction}
\end{table}
